# Supplementary material for: Inverse Design of Potential Singlet Fission Molecules using a Transfer Learning Based Approach
Source: arXiv:2003.07666 ancillary file (2020-03-17)
Supplement: Supplementary file 1 [file Supplementary_Information.pdf]

# Supplementary Information

# Inverse Design of Potential Singlet Fission Molecules using a Transfer Learning Based Approach

Akshay Subramanian[1], Utkarsh Saha[2], Tejasvini Sharma[2], Naveen K. Tailor[2], Soumitra Satapathi[2]

[1] Department of Metallurgical and Materials Engineering, Indian Institute of Technology Roorkee, Roorkee 247667, Uttarakhand, India

[2] Department of Physics, Indian Institute of Technology Roorkee, Roorkee 247667, Uttarakhand, India

# Autoencoder Framework

The autoencoder has an encoder network to convert each SMILES into a fixed-dimensional vector, and a decoder network to convert vectors back into SMILES strings. The autoencoder makes use of a series of transformations to encode the input SMILES string into a compressed continuous representation of each SMILES string, which are subsequently decoded into the original input string. This model is trained to minimize the error in decoding the original string or in other words, learns to reconstruct the original SMILES string. The space represented by this compressed representation (the fixed-dimensional vector) is known as the latent space. The latent space tries to preserve the most statistically important features of the data by acting as an information bottleneck. The encoded vector is known as the latent representation of the molecule. Using traditional autoencoders results in the generation of a large number of invalid SMILES strings since each encoding in the latent space might not correspond to a valid string. To overcome this issue, we used a Variational Autoencoder (VAE) as suggested by Gomez-Bombarelli et al. The VAE improves the probability of generating a valid SMILES string by adding stochasticity to the encoder with the help of a penalty term in order to ensure that every position in the latent space corresponds to a valid molecule. This validity issue is especially important in our case since SMILES strings possess a highly fragile representation and even a minor change in the string sequence can convert a valid SMILES string into an invalid one.

We chose to represent the molecules as SMILES strings so that we could utilize modern advances in the field of Natural Language Processing (NLP) to our problem. We employed the open source cheminformatics suite RDKIT to validate the chemical structures of output molecules and discard invalid ones.

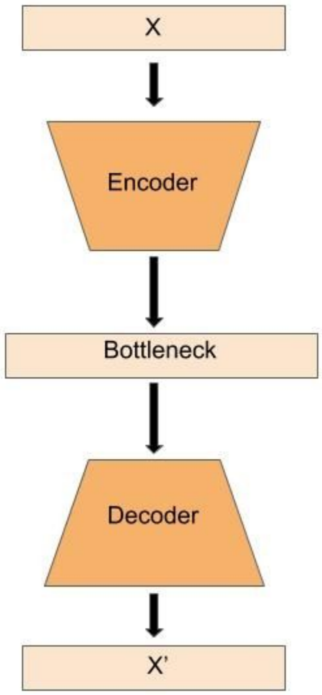


Supplementary Figure 1: A schematic diagram depicting the autoencoder architecture. The input vector X is compressed into a fixed dimensional latent vector by the encoder. The decoder decompresses this latent vector to produce X', which should ideally be the same as X.
